# Supplementary material for: When Fair Ranking Meets Uncertain Inference
Source: arXiv:2105.02091 source file (2022-05-04)
Supplement: Supplementary file 1 [file appendix.tex]

\section*{Appendix}

\subsection{Inference Algorithms}

\subsubsection{EthCNN}

\begin{verbatim}
    {'Asian': {'Asian': 0.408965663416702,
           'Black': 0.05970043803871697,
           'Latinx': 0.030380104564080825,
           'White': 0.5009537939805002},
 'Black': {'Asian': 0.0015337144381331119,
           'Black': 0.3466618978049091,
           'Latinx': 0.004229333753639793,
           'White': 0.647575054003318},
 'Latinx': {'Asian': 0.0035262000454993553,
            'Black': 0.046952807057455574,
            'Latinx': 0.5423649553853542,
            'White': 0.4071560375116908},
 'White': {'Asian': 0.0014619243179104877,
           'Black': 0.04874317059471446,
           'Latinx': 0.006881074128377015,
           'White': 0.9429138309589981}}
\end{verbatim}

\subsubsection{EthniColr}

\begin{verbatim}
    {'Asian': {'Asian': 0.4177458486939534,
           'Black': 0.007971767967986891,
           'Latinx': 0.0795601348583672,
           'White': 0.4947222484796925},
 'Black': {'Asian': 0.1356489679838461,
           'Black': 0.02522582112650309,
           'Latinx': 0.04393063422489593,
           'White': 0.7951945766647549},
 'Latinx': {'Asian': 0.06131009566594049,
            'Black': 0.010202562818830089,
            'Latinx': 0.31740254116882943,
            'White': 0.6110848003464},
 'White': {'Asian': 0.12150850578319809,
           'Black': 0.031444105210971136,
           'Latinx': 0.016651837953604212,
           'White': 0.8303955510522265}}
\end{verbatim}

\subsubsection{BISG}

\begin{verbatim}
    {'Asian': {'Asian': 0.5941320293398533,
           'Black': 0.06601466992665037,
           'Latinx': 0.02444987775061125,
           'White': 0.3154034229828851},
 'Black': {'Asian': 0.0005301825342725138,
           'Black': 0.461334545179126,
           'Latinx': 0.004847383170491555,
           'White': 0.53328788911611},
 'Latinx': {'Asian': 0.0022988505747126436,
            'Black': 0.041379310344827586,
            'Latinx': 0.6781609195402298,
            'White': 0.27816091954022987},
 'White': {'Asian': 0.0010780245708241804,
           'Black': 0.08284517126352615,
           'Latinx': 0.008156374583028233,
           'White': 0.9079204295826214}}
\end{verbatim}

\subsubsection{NamePrism}
\begin{verbatim}
    {'Asian': {'Asian': 0.5155425731351092,
           'Black': 0.003531412128874744,
           'Latinx': 0.05720015695165017,
           'White': 0.4237258577843659},
 'Black': {'Asian': 0.012854789696947564,
           'Black': 0.030497450377013607,
           'Latinx': 0.012174377682485926,
           'White': 0.9444733822435529},
 'Latinx': {'Asian': 0.018531114992186782,
            'Black': 0.006802095780862212,
            'Latinx': 0.4290651714311977,
            'White': 0.5456016177957533},
 'White': {'Asian': 0.007869801118584596,
           'Black': 0.008307528327452463,
           'Latinx': 0.0054088917838486785,
           'White': 0.9784137787701143}}
\end{verbatim}

\subsubsection{DeepFace}
\begin{verbatim}
    {'Asian': {'Asian': 0.614580914789877,
           'Black': 0.15532853494311585,
           'Latinx': 0.06779661016949153,
           'White': 0.16229394009751566},
 'Black': {'Asian': 0.10782380013149244,
           'Black': 0.7238658777120316,
           'Latinx': 0.02827087442472058,
           'White': 0.14003944773175542},
 'Latinx': {'Asian': 0.22010869565217392,
            'Black': 0.14605978260869565,
            'Latinx': 0.32065217391304346,
            'White': 0.313179347826087},
 'White': {'Asian': 0.1185378590078329,
           'Black': 0.07780678851174935,
           'Latinx': 0.10861618798955613,
           'White': 0.6950391644908617}}
\end{verbatim}

\onecolumn

\subsection{Simulations}

\begin{table}[H]
\caption{Simulation NDKL}
\centering
\begin{tabular}{l|rrrrrr}
\toprule
 Accuracy &    Dist A &    Dist B &    Dist C &    Dist D &    Dist E \\
\midrule
       0.1 &  0.079217 &  0.070349 &  0.271969 &  0.324629 &  0.334884 \\
       0.2 &  0.078475 &  0.065082 &  0.234064 &  0.271854 &  0.291437 \\
       0.3 &  0.076075 &  0.060726 &  0.201894 &  0.226753 &  0.246081 \\
       0.4 &  0.074051 &  0.057491 &  0.168142 &  0.186508 &  0.213813 \\
       0.5 &  0.069980 &  0.052763 &  0.145519 &  0.149568 &  0.182016 \\
       0.6 &  0.068764 &  0.049998 &  0.127903 &  0.119351 &  0.148446 \\
      0.7 &  0.064722 &  0.046333 &  0.101726 &  0.096076 &  0.126376 \\
      0.8 &  0.061254 &  0.043500 &  0.090354 &  0.073955 &  0.102914 \\
       0.9 &  0.056751 &  0.039878 &  0.076157 &  0.057676 &  0.085473 \\
       1.0 &  0.052823 &  0.036451 &  0.070669 &  0.047367 &  0.072237 \\
\bottomrule
\end{tabular}
\end{table}

\begin{table}[H]
\caption{Simulation Attention Bias Ratio}
\centering
\begin{tabular}{l|rrrrrr}
\toprule
  Accuracy &    Dist A &    Dist B &    Dist C &    Dist D &    Dist E \\
\midrule
      0.1 &  0.648742 &  0.722814 &  0.841513 &  0.851684 &  0.657778 \\
       0.2 &  0.656772 &  0.743913 &  0.852565 &  0.848273 &  0.667856 \\
      0.3 &  0.669082 &  0.748300 &  0.853303 &  0.844555 &  0.662668 \\
      0.4 &  0.691478 &  0.770209 &  0.861621 &  0.828767 &  0.647317 \\
       0.5 &  0.713418 &  0.794865 &  0.876609 &  0.838288 &  0.663148 \\
      0.6 &  0.736680 &  0.822240 &  0.874840 &  0.842517 &  0.668216 \\
       0.7 &  0.775981 &  0.851826 &  0.868373 &  0.841767 &  0.684981 \\
       0.8 &  0.805954 &  0.882102 &  0.889692 &  0.837325 &  0.701593 \\
       0.9 &  0.868437 &  0.927653 &  0.885315 &  0.860439 &  0.796076 \\
      1.0 &  0.935185 &  0.965964 &  0.932420 &  0.916881 &  0.915150 \\
\bottomrule
\end{tabular}
\end{table}

\begin{table}[H]
\caption{Simulation Disparate Treatment Bias Ratio}
\centering
\begin{tabular}{l|rrrrrr}
\toprule
  Accuracy &    Dist A &    Dist B &    Dist C &    Dist D &    Dist E \\
\midrule
      0.1 &  0.657341 &  0.725589 &  0.844780 &  0.858089 &  0.666002 \\
      0.2 &  0.665277 &  0.742207 &  0.851714 &  0.854265 &  0.675822 \\
      0.3 &  0.677708 &  0.743644 &  0.848992 &  0.852841 &  0.670608 \\
     0.4 &  0.699862 &  0.761614 &  0.853925 &  0.840157 &  0.656134 \\
      0.5 &  0.721609 &  0.782403 &  0.868661 &  0.847945 &  0.671375 \\
      0.6 &  0.745029 &  0.807110 &  0.865899 &  0.859755 &  0.675311 \\
      0.7 &  0.783986 &  0.831957 &  0.862952 &  0.850835 &  0.690747 \\
       0.8 &  0.813688 &  0.863523 &  0.883846 &  0.853317 &  0.707326 \\
       0.9 &  0.875495 &  0.913248 &  0.884281 &  0.874967 &  0.805837 \\
       1.0 &  0.944031 &  0.991223 &  0.959117 &  0.981519 &  0.926947 \\
\bottomrule
\end{tabular}
\end{table}

\begin{table}[H]
\caption{Simulation Disparate Impact Bias Ratio}
\centering
\begin{tabular}{l|rrrrrr}
\toprule
  Accuracy &    Dist A &    Dist B &    Dist C &    Dist D &    Dist E \\
\midrule
       0.1 &  0.644798 &  0.719004 &  0.839626 &  0.847989 &  0.648500 \\
      0.2 &  0.652811 &  0.741219 &  0.851772 &  0.844175 &  0.658246 \\
      0.3 &  0.664916 &  0.746658 &  0.853763 &  0.839482 &  0.654089 \\
      0.4 &  0.687099 &  0.769755 &  0.863757 &  0.822378 &  0.638774 \\
       0.5 &  0.708916 &  0.795945 &  0.878297 &  0.832087 &  0.654594 \\
      0.6 &  0.731846 &  0.824343 &  0.876386 &  0.832776 &  0.659952 \\
       0.7 &  0.770911 &  0.855446 &  0.867998 &  0.833854 &  0.677822 \\
      0.8 &  0.800567 &  0.885890 &  0.888164 &  0.825988 &  0.695157 \\
      0.9 &  0.862909 &  0.929176 &  0.880898 &  0.846256 &  0.785146 \\
     1.0 &  0.928200 &  0.955091 &  0.915843 &  0.886665 &  0.885478 \\
\bottomrule
\end{tabular}
\end{table}

\subsection{Case Studies}

All experiments were done 100 times to control for differences in probabilistic predictions. These are the median values over 100 simulations.

\textbf{A. UCI Income dataset. Size: 7395. Fairness results shown below are for top 300.}

\begin{table}[H]
\caption{Income Dataset Skew}
  \centering
%   \resizebox{\columnwidth}{!}{%
\begin{tabular}{lrrrrrr|l}
\toprule
{} &  Black Women &  Asian Men &  Asian Women &  White Men &  White Women &  Black Men &      NDKL \\
\midrule
Baseline  &    1.301955 &      0.153125 &      0.714523 &      0.499242 &    0.340483 &    2.083042 &  0.209139 \\
Oracle    &    1.013238 &      0.995186 &      0.714523 &      0.998481 &    0.953316 &    0.867965 &  0.049886 \\
EthCnn    &    1.045214 &      0.631569 &      1.407507 &      1.033553 &    0.170610 &    1.866064 &  0.101861 \\
EthniColr &    1.067549 &      0.466984 &      0.680683 &      1.086971 &    0.161914 &    1.163055 &  0.110460 \\
BISG      &    1.066078 &      0.533584 &      1.211043 &      1.056393 &    0.076008 &    1.480711 &  0.107098 \\
Nameprism &    1.061121 &      0.682093 &      1.010393 &      1.039543 &    0.143607 &    1.435579 &  0.097942 \\
DeepFace  &    1.222803 &      0.232769 &      0.486649 &      0.822624 &    0.155333 &    0.657930 &  0.144990 \\
\bottomrule
\end{tabular}
% }
\end{table}

\begin{table}[H]
\caption{Income Dataset Attention}
  \centering
\begin{tabular}{lrrrrrr|l}
\toprule
{} &  White Men &  White Women &  Asian Men &  Black Women &  Asian Women &  Black Men &       ABR \\
\midrule
Baseline  &    0.348573 &      0.326841 &    0.157197 &      0.111217 &      0.143360 &    0.029643 &  0.085040 \\
Oracle    &    0.343497 &      0.321459 &    0.254569 &      0.278332 &      0.177524 &    0.290933 &  0.516815 \\
EthCnn    &    0.351381 &      0.323389 &    0.178502 &      0.211896 &      0.239819 &    0.050740 &  0.144402 \\
EthniColr &    0.349636 &      0.317140 &    0.127533 &      0.211170 &      0.317344 &    0.030163 &  0.086269 \\
BISG      &    0.346789 &      0.321664 &    0.191870 &      0.203879 &      0.231010 &    0.023539 &  0.067878 \\
Nameprism &    0.347707 &      0.324725 &    0.153727 &      0.212778 &      0.229856 &    0.153388 &  0.441143 \\
DeepFace  &    0.340048 &      0.316158 &    0.185071 &      0.218350 &      0.213596 &    0.133154 &  0.391575 \\
\bottomrule
\end{tabular}
\end{table}

\begin{table}[H]
\caption{Income Dataset Disparate Treatment}
\centering
\begin{tabular}{lrrrrrr|l}
\toprule
{} &  White Men &  White Women &  Asian Men &  Black Women &  Asian Women &  Black Men &      DTBR \\
\midrule
Baseline  &    0.400888 &      0.376379 &    0.183563 &      0.130266 &      0.166695 &    0.035641 &  0.088904 \\
Oracle    &    0.390045 &      0.388605 &    0.292054 &      0.377746 &      0.206419 &    0.363571 &  0.529218 \\
EthCnn    &    0.399681 &      0.394301 &    0.208107 &      0.278110 &      0.301709 &    0.061077 &  0.152814 \\
EthniColr &    0.400163 &      0.407846 &    0.148654 &      0.279696 &      0.379904 &    0.036306 &  0.089018 \\
BISG      &    0.394817 &      0.391294 &    0.222183 &      0.256275 &      0.283343 &    0.027967 &  0.070836 \\
Nameprism &    0.401288 &      0.422540 &    0.178364 &      0.407245 &      0.279132 &    0.224747 &  0.422123 \\
DeepFace  &    0.395148 &      0.384300 &    0.219415 &      0.283587 &      0.257879 &    0.172006 &  0.435295 \\
\bottomrule
\end{tabular}
\end{table}

\begin{table}[H]
\caption{Income Dataset Disparate Impact}
\centering
\begin{tabular}{lrrrrrr|l}
\toprule
{} &  White Men &  White Women &  Asian Men &  Black Women &  Asian Women &  Black Men &      DIBR \\
\midrule
Baseline  &    0.316067 &      0.293841 &    0.136607 &      0.095413 &      0.123301 &    0.024704 &  0.078162 \\
Oracle    &    0.314211 &      0.282291 &    0.224148 &      0.227083 &      0.152782 &    0.240621 &  0.486240 \\
EthCnn    &    0.320793 &      0.282926 &    0.155169 &      0.173577 &      0.199964 &    0.042257 &  0.131727 \\
EthniColr &    0.317909 &      0.271225 &    0.110970 &      0.171326 &      0.269835 &    0.025050 &  0.078796 \\
BISG      &    0.316508 &      0.281517 &    0.167861 &      0.170351 &      0.195096 &    0.019813 &  0.062598 \\
Nameprism &    0.315550 &      0.272711 &    0.134167 &      0.133985 &      0.194438 &    0.113852 &  0.360806 \\
DeepFace  &    0.306817 &      0.276627 &    0.158606 &      0.178642 &      0.179122 &    0.105718 &  0.344563 \\
\bottomrule
\end{tabular}
\end{table}

% \newpage

\textbf{B. Compas dataset. Size: 6171. Fairness results shown below are for top 300.}

\begin{table}[H]
\caption{Compas Dataset Skew}
\centering
% \resizebox{\columnwidth}{!}{%
\begin{tabular}{lrrrrrr|l}
\toprule
{} &  White Men &  Latino Men &  Black Women &  Latina Women &  Black Men &  White Women &      NDKL \\
\midrule
Baseline  &    0.368904 &     0.451764 &      0.351373 &       0.235298 &    1.785021 &      0.200113 &  0.209139 \\
Oracle    &    1.011505 &     0.993864 &      0.983825 &       0.940980 &    1.006371 &      0.960498 &  0.049886 \\
EthCnn    &    0.183859 &     0.940106 &      1.440596 &       0.868059 &    1.523512 &      0.466248 &  0.101861 \\
EthniColr &    0.766127 &     0.505522 &      1.207995 &       0.534037 &    1.225054 &      0.840838 &  0.110460 \\
BISG      &    0.206707 &     0.928360 &      1.431461 &       0.790434 &    1.513816 &      0.476253 &  0.107098 \\
Nameprism &    0.309404 &     1.027746 &      1.445516 &       0.896287 &    1.411930 &      0.563898 &  0.097942 \\
DeepFace  &    0.538955 &     0.645565 &      0.459593 &       0.378787 &    1.580956 &      0.420625 &  0.144990 \\
\bottomrule
\end{tabular}
% }

\end{table}

\begin{table}[H]
\caption{Compas Dataset Attention}
\centering
\begin{tabular}{lrrrrrr|l}
\toprule
{} &  Black Men &  White Men &  Latino Men &  White Women &  Black Women &  Latina Women &       ABR \\
\midrule
Baseline  &    0.332558 &    0.340952 &     0.301716 &      0.512798 &      0.188167 &       0.082385 &  0.160658 \\
Oracle    &    0.348578 &    0.323225 &     0.310127 &      0.311350 &      0.307135 &       0.200505 &  0.575210 \\
EthCnn    &    0.331793 &    0.440179 &     0.307809 &      0.411868 &      0.279124 &       0.230719 &  0.524148 \\
EthniColr &    0.369293 &    0.266314 &     0.253218 &      0.354658 &      0.277723 &       0.255570 &  0.685683 \\
BISG      &    0.332721 &    0.423985 &     0.299121 &      0.417091 &      0.274884 &       0.249131 &  0.587593 \\
Nameprism &    0.350770 &    0.335751 &     0.236233 &      0.387410 &      0.276100 &       0.211608 &  0.546213 \\
DeepFace  &    0.345156 &    0.298206 &     0.294533 &      0.374866 &      0.213606 &       0.246038 &  0.569820 \\
\bottomrule
\end{tabular}

\end{table}

\begin{table}[H]
\caption{Compas Dataset Disparate Treatment}
\centering
\begin{tabular}{lrrrrrr|l}
\toprule
{} &  Black Men &  White Men &  Latino Men &  White Women &  Black Women &  Latina Women &      DTBR \\
\midrule
Baseline  &    0.366816 &    0.377640 &     0.333884 &      0.557392 &      0.211857 &       0.092734 &  0.166372 \\
Oracle    &    0.373015 &    0.386776 &     0.365779 &      0.408358 &      0.371788 &       0.300697 &  0.736357 \\
EthCnn    &    0.370030 &    0.477108 &     0.378196 &      0.495242 &      0.365025 &       0.332882 &  0.672160 \\
EthniColr &    0.481002 &    0.523903 &     0.351276 &      0.619709 &      0.414737 &       0.352704 &  0.566840 \\
BISG      &    0.366328 &    0.457890 &     0.358567 &      0.499325 &      0.352151 &       0.343290 &  0.687507 \\
Nameprism &    0.457754 &    0.500106 &     0.316098 &      0.538359 &      0.423861 &       0.317853 &  0.587152 \\
DeepFace  &    0.381197 &    0.342831 &     0.336803 &      0.443325 &      0.250377 &       0.285686 &  0.564769 \\
\bottomrule
\end{tabular}

\end{table}

\begin{table}[H]
\caption{Compas Dataset Disparate Impact}
\centering
\begin{tabular}{lrrrrrr|l}
\toprule
{} &  Black Men &  White Men &  Latino Men &  White Women &  Black Women &  Latina Women &      DIBR \\
\midrule
Baseline  &    0.314294 &    0.324632 &     0.284676 &      0.487827 &      0.173729 &       0.073191 &  0.150034 \\
Oracle    &    0.334369 &    0.291903 &     0.282491 &      0.270766 &      0.271961 &       0.166037 &  0.496569 \\
EthCnn    &    0.311970 &    0.423545 &     0.274091 &      0.377808 &      0.234040 &       0.186148 &  0.439499 \\
EthniColr &    0.311814 &    0.196970 &     0.217381 &      0.271737 &      0.203934 &       0.208851 &  0.631690 \\
BISG      &    0.314716 &    0.408306 &     0.270215 &      0.382681 &      0.233885 &       0.206071 &  0.504697 \\
Nameprism &    0.284102 &    0.274905 &     0.202045 &      0.327184 &      0.184841 &       0.164303 &  0.502172 \\
DeepFace  &    0.325627 &    0.278434 &     0.272377 &      0.344317 &      0.191131 &       0.214222 &  0.555104 \\
\bottomrule
\end{tabular}

\end{table}

\begin{table}[H]
\caption{Notations used}
\centering
\begin{tabular}{c|C{9cm}|C{5cm}}
\toprule
\textbf{Symbol}  &  \textbf{Definition} &  \textbf{Interpretation} \\
\midrule
\midrule

% $\tau$ & A ranked list & --- \\
$\text{Skew}_{g_{i}}@k(\tau)$  &    $\frac{\text{\% of members $\in$ group $g_{i}$ in the top $k$ items in $\tau$}}{\text{\% of members $\in$ group $g_{i}$ in the overall population $q$}}$
 &   \makecell{ 1 : fair
 \\ $>$ 1 : overrepresentation of $g_i$ 
 \\ $<$ 1 : underrepresentation of $g_i$ }   \\
\midrule

$ \text{NDKL}(\tau)$ & The normalized discounted KL divergence between top $k$ elements and overall population $q$ & \makecell{0 is perfectly fair\\lower is better}\\ 
\midrule

$\eta_{g_{j}},\tau$ & The mean attention provided to each member of group $g_i$ in $\tau$
& higher is better \\
\midrule

$U_{g_{j},\tau}$ & The mean utility score for each member of group $g_i$ in $\tau$
& higher is better \\
\midrule

$\theta_{\tau, g_{j}}$ & The mean attention weighted by mean utility for group $g_i$ in $\tau$  & higher is better\\

\midrule

$\gamma_{\tau, g_{j}}$ & The mean action rate per member for group $g_i$ in $\tau$  & higher is better\\

\midrule

$ \text{ABR}_{\tau} $ & The ratio of minimum $\eta_{g_{j}}$ to maximum $\eta_{g_{j}}$ for $\tau$  & \makecell{1 is perfectly fair\\lower suggests more disparity}\\
\midrule

$ \text{DTBR}_{\tau}$ & The ratio of minimum $\theta_{g_{j}}$ to maximum $\theta_{g_{j}}$ for $\tau$  & \makecell{1 is perfectly fair\\lower suggests more disparity}\\
\midrule

$ \text{DIBR}_{\tau}$ & The ratio of minimum $\gamma_{g_{j}}$ to maximum $\gamma_{g_{j}}$ for $\tau$  & \makecell{1 is perfectly fair\\lower suggests more disparity}\\

\bottomrule
\end{tabular}

\end{table}

\twocolumn
