# Supplementary material for: When Fair Ranking Meets Uncertain Inference
Source: arXiv:2105.02091 source file (2022-05-04)
Supplement: Supplementary file 2 [file supplementary.tex]

\section*{Supplementary Material}
